# Supplementary material for: Time Series Classification Using Convolutional Neural Network On Imbalanced Datasets
Source: arXiv:2110.04748 source file (2021-10-10)
Supplement: Supplementary file 1 [file appendix.tex]

% !TeX spellcheck = en_US
% !TeX encoding = UTF-8
\chapter{Code}
how you make the ds imbalance
\chapter{Math}

\chapter{Dataset}
